# Supplementary material for: QCD field-strength correlators on a Polyakov loop with gradient flow at next-to-leading order
Source: arXiv:2410.01578 source file (2024-10-02)
Supplement: Supplementary file 1 [file appendixexpressions.tex]

\subsection{Electric correlator}

\begin{widetext}

\begin{equation}
\delta_{(a)}G_{E}^{(4)}\left(\tau,\tauf\right)=\left(\frac{g_{B}^{2}}{3}-\frac{1}{3\epsilon}\frac{g_{B}^{4}}{\left(4\pi\right)^{2}}\left(\frac{11\CA-4N_{f}T_{f}}{3}\right)\right)\mu^{4-D}\CR\mbox{Re}\int_{P}\left(1+\frac{\left(D-2\right)p_{0}^{2}}{P^{2}}\right)e^{ip_{0}\tau}e^{-2\taufP^{2}}.
\end{equation}

\begin{equation}
\begin{array}{c}
\delta_{(b-f)}G_{E}^{(4)}\left(\tau,\tauf\right)=-\frac{g_{B}^{4}}{6}\CA\CR\mbox{Re}\int_{P}\left(1+\left(D-2\right)\frac{p_{0}^{2}}{P^{2}}\right)e^{ip_{0}\tau}e^{-2\taufP^{2}}\times
\\
\\
\int_{K}\left(\int_{\tau}^{\infty}ds_{1}\int_{0}^{\tau}ds_{2}+\int_{0}^{\tau}ds_{1}\int_{-\infty}^{0}ds_{2}\right)e^{ik_{0}(s_{1}-s_{2})}\frac{e^{-2\taufK^{2}}}{K^{2}}.
\end{array}
\end{equation}

\begin{equation}
\begin{array}{c}
\delta_{(g)}G_{E}^{(4)}\left(\tau,\tauf\right)=\frac{g_{B}^{4}}{6}\CA\CR\left(D-1\right)\mbox{Re}\int_{P}ip_{0}e^{ip_{0}\tau}\frac{e^{-2\taufP^{2}}}{P^{2}}\times
\\
\\
\int_{K}\frac{e^{-2\taufK^{2}}}{K^{2}}\left(\int_{-\infty}^{\infty}ds-2\int_{0}^{\tau}ds\right)e^{ik_{0}s}\left(1+e^{-ik_{0}\tau}\right).
\end{array}
\end{equation}

\begin{equation}
\delta_{(h)}G_{E}^{(4)}\left(\tau,\tauf\right)=-\frac{g_{B}^{4}}{3}\CA\CR\left(D-1\right)\mbox{Re}\int_{P,K}e^{i(p_{0}+k_{0})\tau}\frac{e^{-2\tauf(P^{2}+K^{2})}}{P^{2}K^{2}}.
\end{equation}

\begin{equation}
\delta_{(i_{1})}G_{E}^{(4)}\left(\tau,\tauf\right)=g_{B}^{4}\CA\CR\mbox{Re}\int_{P}e^{ip_{0}\tau}e^{-2\taufP^{2}}\left(1+\left(D-2\right)\frac{p_{0}^{2}}{P^{2}}\right)\int_{K}\frac{e^{-\tauf(K^{2}+(P+K)^{2}-P^{2})}}{K^{2}\left(P+K\right)^{2}}.
\end{equation}

\begin{equation}
\begin{array}{c}
\delta_{(i_{2})}G_{E}^{(4)}\left(\tau,\tauf\right)=\frac{2}{3}g_{B}^{4}\CA\CR\mbox{Re}\int_{0}^{\tauf}ds\int_{P,K}e^{ip_{0}\tau}\frac{e^{-(\tauf+s)(P^{2}+K^{2})}}{P^{2}K^{2}}e^{-(\tauf-s)(P+K)^{2}}
\\
\\
\times\left[3\left(P^{2}+\left(D-2\right)p_{0}^{2}\right)+\frac{1}{2}\left(K^{2}+P^{2}-\left(P+K\right)^{2}\right)-\left(D-2\right)p_{0}k_{0}\right].
\end{array}
\end{equation}

\begin{equation}
\delta_{(i_{3})}G_{E}^{(4)}\left(\tau,\tauf\right)=\frac{2}{3}g_{B}^{4}\CA\CR\mbox{Re}\int_{0}^{\tauf}ds\int_{P,K}\left(P^{2}+\left(D-2\right)p_{0}^{2}\right)e^{ip_{0}\tau}\frac{e^{-(\tauf+s)(K^{2}+(P+K)^{2})}}{K^{2}\left(P+K\right)^{2}}e^{-(\tauf-s)P^{2}}.
\end{equation}

\begin{equation}
\begin{array}{c}
\delta_{(j_{1})}G_{E}^{(4)}\left(\tau,\tauf\right)=-\frac{g_{B}^{4}}{6}\CA\CR\mbox{Re}\left(\int_{-\infty}^{\infty}ds-2\int_{0}^{\tau}ds\right)\int_{P,K}ie^{ip_{0}\tau}e^{ik_{0}s}\frac{e^{-\tauf(P^{2}+K^{2}+(P+K)^{2})}}{P^{2}K^{2}\left(P+K\right)^{2}}
\\
\\
\times\left[p_{0}\left(\left(D-1\right)\left(3p_{0}k_{0}+k_{0}^{2}+2p_{0}^{2}\right)+2\left(\vec{p}^{2}+\vec{p}\cdot\vec{k}+\vec{k}^{2}\right)\right)+k_{0}\left(\vec{p}^{2}-\vec{p}\cdot\vec{k}\right)\right].
\end{array}
\end{equation}

\begin{equation}
\begin{array}{c}
\delta_{(j_{2})}G_{E}^{(4)}\left(\tau,\tauf\right)=-\frac{g_{B}^{4}}{3}\CA\CR\mbox{Re}\left(\int_{-\infty}^{\infty}ds-2\int_{0}^{\tau}ds\right)\int_{0}^{\tauf}ds_{1}\int_{P,K}e^{ip_{0}\tau}e^{ik_{0}s}\frac{e^{-(\tauf+s_{1})(P^{2}+K^{2})}}{P^{2}K^{2}}\times
\\
\\
e^{-(\tauf-s_{1})(P+K)^{2}}\left[p_{0}\left(P^{2}+K^{2}+\left(P+K\right)^{2}\right)+k_{0}\left(P^{2}+K^{2}-\left(P+K\right)^{2}\right)+2\left(D-2\right)p_{0}^{2}\left(p_{0}+k_{0}\right)\right].
\end{array}
\end{equation}

\begin{equation}
\begin{array}{c}
\delta_{(j_{3})}G_{E}^{(4)}\left(\tau,\tauf\right)=-\frac{g_{B}^{4}}{6}\CA\CR\mbox{Re}\left(\int_{-\infty}^{\infty}ds-2\int_{0}^{\tau}ds\right)\int_{0}^{\tauf}ds_{1}\int_{P,K}e^{ip_{0}\tau}e^{ik_{0}s}\frac{e^{-(\tauf+s_{1})(P^{2}+(P+K)^{2})}}{P^{2}\left(P+K\right)^{2}}e^{-(\tauf-s_{1})K^{2}}
\\
\\
\times\left[\left(D-2\right)p_{0}\left(p_{0}+k_{0}\right)\left(2p_{0}+k_{0}\right)+\frac{k_{0}}{2}\left(3P^{2}+K^{2}-\left(P+K\right)^{2}\right)+p_{0}\left(P^{2}+K^{2}+\left(P+K\right)^{2}\right)\right].
\end{array}
\end{equation}

\begin{equation}
\delta_{(k_{1}-k_{4})}G_{E}^{(4)}\left(\tau,\tauf\right)=\frac{g_{B}^{2}}{3}\CR\int_{P}e^{ip_{0}\tau}e^{-2\taufP^{2}}\left(1+\left(D-2\right)\frac{p_{0}^{2}}{P^{2}}\right)\frac{\Pi_{\alpha\beta}\left(P\right)}{P^{2}},
\end{equation}

where

\begin{equation}
\begin{array}{c}
\Pi_{\alpha\beta}^{\mbox{\scriptsize{(boson)}}}\left(P\right)=-g_{B}^{2}\mathcal{C}_{A}\frac{\Gamma\left(2-\frac{D}{2}\right)\Gamma\left(\frac{D}{2}-1\right)\Gamma\left(\frac{D}{2}\right)}{\left(4\pi\right)^{\frac{D}{2}}\Gamma\left(D\right)}\mu^{4-D}\left(3D-2\right)\left(P^{2}\right)^{\frac{D}{2}-2}\left(\delta_{\alpha\beta}P^{2}-P_{\alpha}P_{\beta}\right).\\
\\
\Pi_{\alpha\beta}^{\mbox{\scriptsize{(fermion)}}}\left(P\right)=8g_{B}^{2}N_{f}T_{f}\frac{\Gamma\left(2-\frac{D}{2}\right)\Gamma^{2}\left(\frac{D}{2}\right)}{\left(4\pi\right)^{\frac{D}{2}}\Gamma\left(D\right)}\mu^{4-D}\left(P^{2}\right)^{\frac{D}{2}-2}\left(\delta_{\alpha\beta}P^{2}-P_{\alpha}P_{\beta}\right).
\end{array}
\label{B-F self-energy tensor}
\end{equation}

\begin{equation}
\delta_{(k_{5})}G_{E}^{(4)}\left(\tau,\tauf\right)=-\frac{g_{B}^{4}}{3}\CA\CR\left(D-1\right)\int_{P}e^{ip_{0}\tau}e^{-2\taufP^{2}}\left(1+\left(D-2\right)\frac{p_{0}^{2}}{P^{2}}\right)\int_{K}\frac{\left(e^{-2\taufK^{2}}-1\right)}{\left(K^{2}\right)^{2}}.
\end{equation}

\begin{equation}
\begin{array}{c}
\delta_{(k_{6})}G_{E}^{(4)}\left(\tau,\tauf\right)=-\frac{2}{3}g_{B}^{4}\frac{\mathcal{C}_{A}\CR}{D-1}\int_{0}^{\tauf}ds_{1}\int_{0}^{s_{1}}ds_{2}\int_{P,K}e^{ip_{0}\tau}e^{-2\taufP^{2}}\left(1+\left(D-2\right)\frac{p_{0}^{2}}{P^{2}}\right)\frac{e^{-(s_{1}+s_{2})\left(P+K\right)^{2}}}{\left(P+K\right)^{2}}
\\
\\
\times e^{-(s_{2}-s_{1})(P^{2}-K^{2})}\left[\left(5D-9\right)K^{2}+\left(D-1\right)\left(3P^{2}+\left(P+K\right)^{2}\right)-\left(4D-8\right)\frac{\left(P\cdot K\right)^{2}}{P^{2}}\right].
\end{array}
\end{equation}

\begin{equation}
\begin{array}{c}
\delta_{(k_{7})}G_{E}^{(4)}\left(\tau,\tauf\right)=\frac{2}{3}g_{B}^{4}\frac{\mathcal{C}_{A}\CR}{D-1}\int_{0}^{\tauf}ds\int_{P,K}e^{ip_{0}\tau}e^{-2\taufP^{2}}\left(1+\left(D-2\right)\frac{p_{0}^{2}}{P^{2}}\right)\times
\\
\frac{e^{-s(K^{2}+\left(P+K\right)^{2}-P^{2}}}{K^{2}\left(P+K\right)^{2}}\left[\left(6-4D\right)\left(P+K\right)^{2}-\left(D-1\right)P^{2}+\left(2D-4\right)\frac{\left(P\cdot K\right)^{2}}{P^{2}}\right].
\end{array}
\end{equation}

\begin{equation}
\begin{array}{c}
\delta_{(k_{8})}G_{E}^{(4)}\left(\tau,\tauf\right)=\frac{1}{6}g_{B}^{4}\frac{\CA\CR}{D-1}\int_{0}^{\tauf}ds_{1}\int_{0}^{\tauf}ds_{2}\int_{P,K}e^{ip_{0}\tau}e^{-2\taufP^{2}}\left(P^{2}+\left(D-2\right)p_{0}^{2}\right)
\\
\\
\times\frac{e^{-(s_{1}+s_{2})(K^{2}+\left(P+K\right)^{2}-P^{2}})}{K^{2}\left(P+K\right)^{2}}\left[-\left(12D-16\right)\left(P+K\right)^{2}+\left(4D-8\right)\frac{\left(P\cdot K\right)^{2}}{P^{2}}\right].
\end{array}
\end{equation}

\subsection{Magnetic correlator}

\begin{equation}
\delta_{(a)}G_{H}^{(2)}\left(\tau,\tauf\right)=\left(\frac{g_{B}^{2}}{3}-\frac{1}{3\epsilon}\frac{g_{B}^{4}}{\left(4\pi\right)^{2}}\left(\frac{11\CA-4N_{f}T_{f}}{3}\right)\right)\left(D-2\right)\mu^{4-D}\CR\int_{P}\left(1-\frac{p_{0}^{2}}{P^{2}}\right)e^{ip_{0}\tau}e^{-2\taufP^{2}}.
\end{equation}

\begin{equation}
\begin{array}{c}
\delta_{(b-f)}G_{H}^{(4)}\left(\tau,\tauf\right)=g_{B}^{4}\frac{\left(D-2\right)}{6}\CA\CR\mbox{Re}\int_{P}\left(1-\frac{p_{0}^{2}}{P^{2}}\right)e^{ip_{0}\tau}e^{-2\taufP^{2}}\times\\
\\
\int_{K}\left(\int_{\tau}^{\infty}ds_{1}\int_{0}^{\tau}ds_{2}+\int_{0}^{\tau}ds_{1}\int_{-\infty}^{0}ds_{2}\right)e^{ik_{0}(s_{1}-s_{2})}\frac{e^{-2\taufK^{2}}}{K^{2}}.
\end{array}
\end{equation}

\begin{equation}
\delta_{(g)}G_{H}^{(4)}\left(\tau,\tauf\right)=0.
\end{equation}
\\

\begin{equation}
\delta_{(h)}G_{H}^{(4)}\left(\tau,\tauf\right)=g_{B}^{4}\frac{\left(D-2\right)\left(D-1\right)}{6}\CA\CR\mbox{Re}\int_{P,K}e^{i(p_{0}+k_{0})\tau}\frac{e^{-2\tauf(P^{2}+K^{2})}}{P^{2}K^{2}}.
\end{equation}

\begin{equation}
\delta_{(i_{1})}G_{H}^{(4)}\left(\tau,\tauf\right)=-g_{B}^{4}\left(D-2\right)\CA\CR\mbox{Re}\int_{P}e^{ip_{0}\tau}e^{-\taufP^{2}}\left(1-\frac{p_{0}^{2}}{P^{2}}\right)\int_{K}\frac{e^{-\tauf(K^{2}+(P+K)^{2})}}{K^{2}\left(P+K\right)^{2}}.
\end{equation}

\begin{equation}
\delta_{(i_{2})}G_{H}^{(4)}\left(\tau,\tauf\right)=-\frac{2}{3}g_{B}^{4}\left(D-2\right)\CA\CR\mbox{Re}\int_{0}^{\tauf}ds\int_{P,K}e^{ip_{0}\tau}\frac{e^{-(\tauf+s)(P^{2}+K^{2})}}{P^{2}K^{2}}e^{-(\tauf-s)(P+K)^{2}}\left(3\vec{p}^{2}-\vec{p}\cdot\vec{k}\right).
\end{equation}

\begin{equation}
\delta_{(i_{3})}G_{H}^{(4)}\left(\tau,\tauf\right)=-\frac{2}{3}g_{B}^{4}\left(D-2\right)\CA\CR\mbox{Re}\int_{0}^{\tauf}ds\int_{P,K}e^{ip_{0}\tau}\frac{e^{-(\tauf+s)(K^{2}+(P+K)^{2})}}{K^{2}\left(P+K\right)^{2}}e^{-(\tauf-s)P^{2}}\vec{p}^{2}.
\end{equation}

\begin{equation}
\begin{array}{c}
\delta_{(j_{1})}G_{H}^{(4)}\left(\tau,\tauf\right)=g_{B}^{4}\frac{\left(D-2\right)}{6}\CA\CR\mbox{Re}\left(\int_{-\infty}^{\infty}ds-2\int_{0}^{\tau}ds\right)\int_{P,K}ie^{ip_{0}\tau}\times\\
\\
e^{ik_{0}s}\frac{e^{-\tauf(P^{2}+K^{2}+(P+K)^{2})}}{P^{2}K^{2}\left(P+K\right)^{2}}\left(2p_{0}+k_{0}\right)\left(\vec{p}^{2}+\vec{p}\cdot\vec{k}\right).
\end{array}
\end{equation}

\begin{equation}
\begin{array}{c}
\delta_{(j_{2})}G_{H}^{(4)}\left(\tau,\tauf\right)=\frac{2}{3}g_{B}^{4}\left(D-2\right)\CA\CR\mbox{Re}\left(\int_{-\infty}^{\infty}ds-2\int_{0}^{\tau}ds\right)\int_{0}^{\tauf}ds_{1}\\
\\
\times\int_{P,K}ie^{ip_{0}\tau}e^{ik_{0}s}\frac{e^{-(\tauf+s_{1})(P^{2}+K^{2})}}{P^{2}K^{2}}e^{-(\tauf-s_{1})(P+K)^{2}}p_{0}\left(\vec{p}^{2}+\vec{p}\cdot\vec{k}\right).
\end{array}
\end{equation}

\begin{equation}
\begin{array}{c}
\delta_{(j_{3})}G_{H}^{(4)}\left(\tau,\tauf\right)=g_{B}^{4}\frac{\left(D-2\right)}{6}\CA\CR\mbox{Re}\left(\int_{-\infty}^{\infty}ds-2\int_{0}^{\tau}ds\right)\int_{0}^{\tauf}ds_{1}\\
\\
\times\int_{P,K}ie^{ip_{0}\tau}e^{ik_{0}s}\frac{e^{-(\tauf+s_{1})(P^{2}+(P+K)^{2})}}{P^{2}\left(P+K\right)^{2}}e^{-(\tauf-s_{1})K^{2}}\left(2p_{0}+k_{0}\right)\left(\vec{p}^{2}+\vec{p}\cdot\vec{k}\right).
\end{array}
\end{equation}

\begin{equation}
\delta_{(k_{1}-k_{4})}G_{H}^{(4)}\left(\tau,\tauf\right)=-g_{B}^{2}\CR\frac{\epsilon_{ijk}\epsilon_{ilm}}{12}\mbox{Re}\int_{P}e^{ip_{0}\tau}\frac{e^{-2\taufP^{2}}}{P^{2}}\left(p_{j}\delta_{k\alpha}-p_{k}\delta_{j\alpha}\right)\left(p_{l}\delta_{m\beta}-p_{m}\delta_{l\beta}\right)\frac{\Pi_{\alpha\beta}\left(P\right)}{P^{2}},
\end{equation}

\begin{equation}
\delta_{(k_{5})}G_{H}^{(4)}\left(\tau,\tauf\right)=g_{B}^{4}\frac{\left(D-2\right)\left(D-1\right)}{3}\CA\CR\mbox{Re}\int_{P}e^{ip_{0}\tau}e^{-2\taufP^{2}}\left(1-\frac{p_{0}^{2}}{P^{2}}\right)\int_{K}\frac{\left(e^{-2\taufK^{2}}-1\right)}{\left(K^{2}\right)^{2}}.
\end{equation}

\begin{equation}
\begin{array}{c}
\delta_{(k_{6})}G_{H}^{(4)}\left(\tau,\tauf\right)=\frac{2}{3}g_{B}^{4}\left(\frac{D-2}{D-1}\right)\mathcal{C}_{A}\CR\mbox{Re}\int_{0}^{\tauf}ds_{1}\int_{0}^{s_{1}}ds_{2}\int_{P,K}e^{ip_{0}\tau}e^{-2\taufP^{2}}\left(1-\frac{p_{0}^{2}}{P^{2}}\right)\times
\\
\\
\frac{e^{-2s_{1}K^{2}-2(s_{2}-s_{1})P\cdot K}}{K^{2}}\left[\left(4D-4\right)P^{2}+\left(6D-10\right)K^{2}-\left(2D-2\right)\left(P\cdot K\right)-\left(4D-8\right)\frac{\left(P\cdot K\right)^{2}}{P^{2}}\right].
\end{array}
\end{equation}

\begin{equation}
\begin{array}{c}
\delta_{(k_{7})}G_{H}^{(4)}\left(\tau,\tauf\right)=-\frac{2}{3}g_{B}^{4}\left(\frac{D-2}{D-1}\right)\CA\CR\mbox{Re}\int_{0}^{\tauf}ds\int_{P,K}e^{ip_{0}\tau}e^{-2\taufP^{2}}\left(1-\frac{p_{0}^{2}}{P^{2}}\right)\times
\\
\\
\frac{e^{-2s(K^{2}+P\cdot K)}}{K^{2}\left(P+K\right)^{2}}\left[\left(6-4D\right)\left(P+K\right)^{2}-\left(D-1\right)P^{2}+2\left(D-2\right)\frac{\left(P\cdot K\right)^{2}}{P^{2}}\right].
\end{array}
\end{equation}

\begin{equation}
\begin{array}{c}
\delta_{(k_{8})}G_{H}^{(4)}\left(\tau,\tauf\right)=-\frac{1}{6}g_{B}^{4}\left(\frac{D-2}{D-1}\right)\CA\CR\mbox{Re}\int_{0}^{\tauf}ds_{1}\int_{0}^{\tauf}ds_{2}\int_{P,K}e^{ip_{0}\tau}e^{-2\taufP^{2}}\left(P^{2}-p_{0}^{2}\right)\times
\\
\\
\frac{e^{-(s_{1}+s_{2})(2K^{2}+2P\cdot K)}}{K^{2}\left(P+K\right)^{2}}\left[-4\left(3D-4\right)\left(P+K\right)^{2}+4\left(D-2\right)\frac{\left(P\cdot K\right)^{2}}{P^{2}}\right].
\end{array}
\end{equation}

\end{widetext}
